# Supplementary material for: Learning Design and Construction with Varying-Sized Materials via Prioritized Memory Resets
Source: arXiv:2204.05509 source file (2022-04-12)
Supplement: Supplementary file 1 [file appendix.tex]

\subsection{Implementation details}
The hyperparamters for training the high-level designer are listed in Table~\ref{tab:app:hyperparameters}.
\begin{table}[h]
    \caption{Hyperparamters for training PPG with {\name}.}
    \label{tab:app:hyperparameters}
    \centering
    \begin{tabular}{cc}
    \toprule
        Hyperparamter & Value \\
    \midrule
        $p_{restart}$ & 0.5 \\
        $\gamma$ & 0.97 \\
        $\epsilon$ & 0.2 \\
        $\beta_{aux}$ & 0.1 \\
        $\beta_{clone}$ & 1 \\
        n\_iters & 300 \\
        n\_steps & 1024 \\
        n\_minibatchs & 32 \\
    \bottomrule
    \end{tabular}
\end{table}
\hide{
\subsection{Additional results}\label{sec:app:results}
\begin{figure*}
    \centering
    \begin{minipage}{0.9\textwidth}
        \begin{subfigure}[t]{\linewidth}
            \centering
            \includegraphics[width=\linewidth]{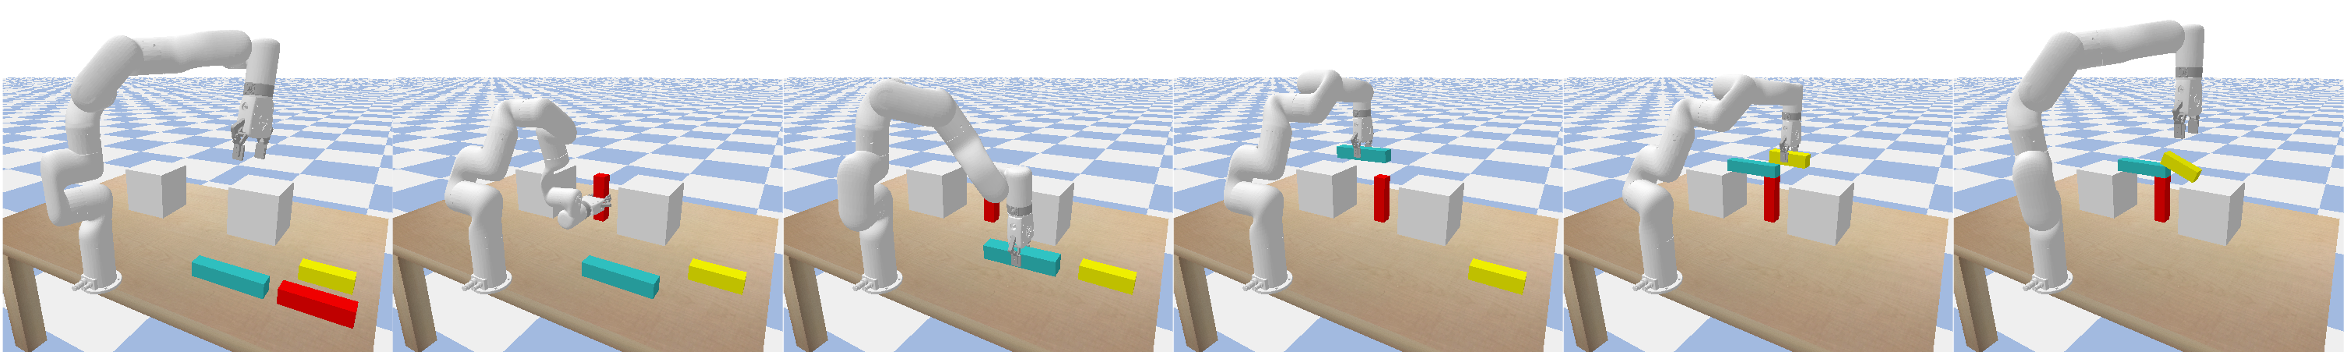}
            \includegraphics[width=\linewidth]{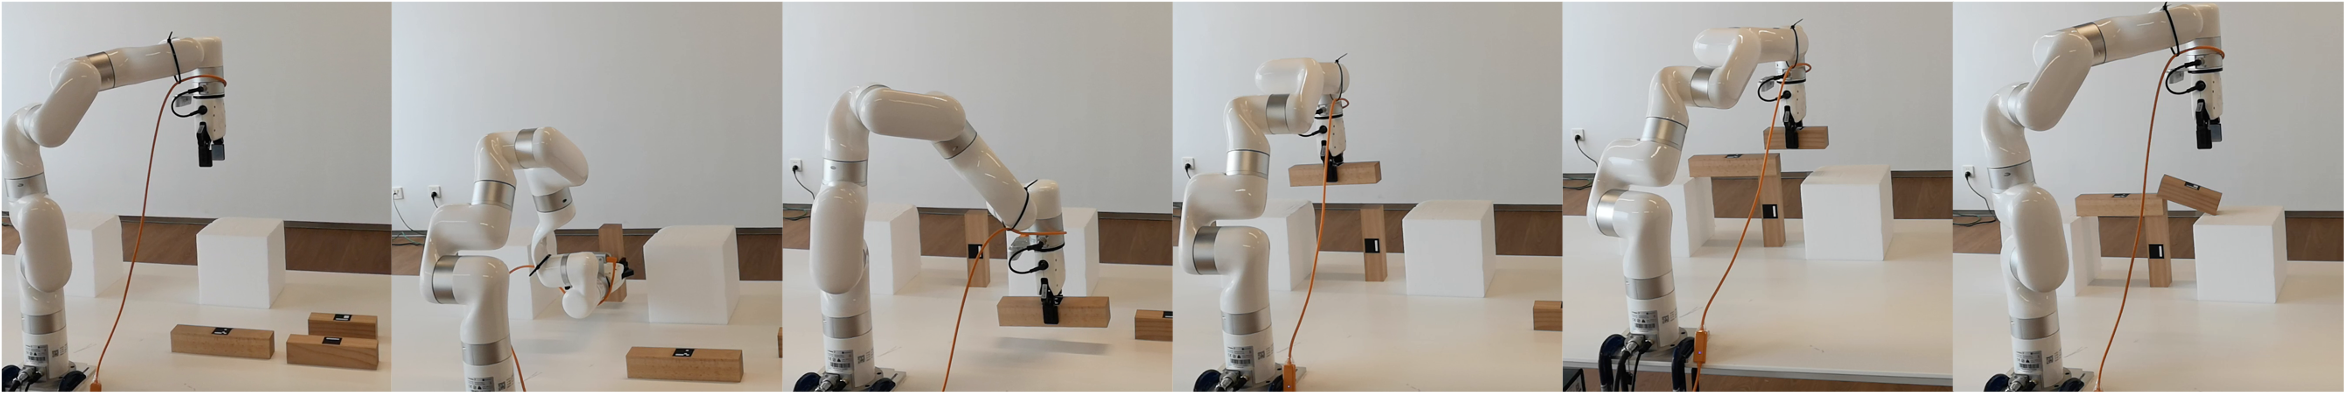}
            % \caption{Learned strategy for building a bridge using 3 blocks with different lengths.}
            % \label{fig:policy_3b}
        \end{subfigure}
    \end{minipage}
    \begin{minipage}{0.9\textwidth}
        \begin{subfigure}[t]{\linewidth}
            \centering
            \includegraphics[width=\linewidth]{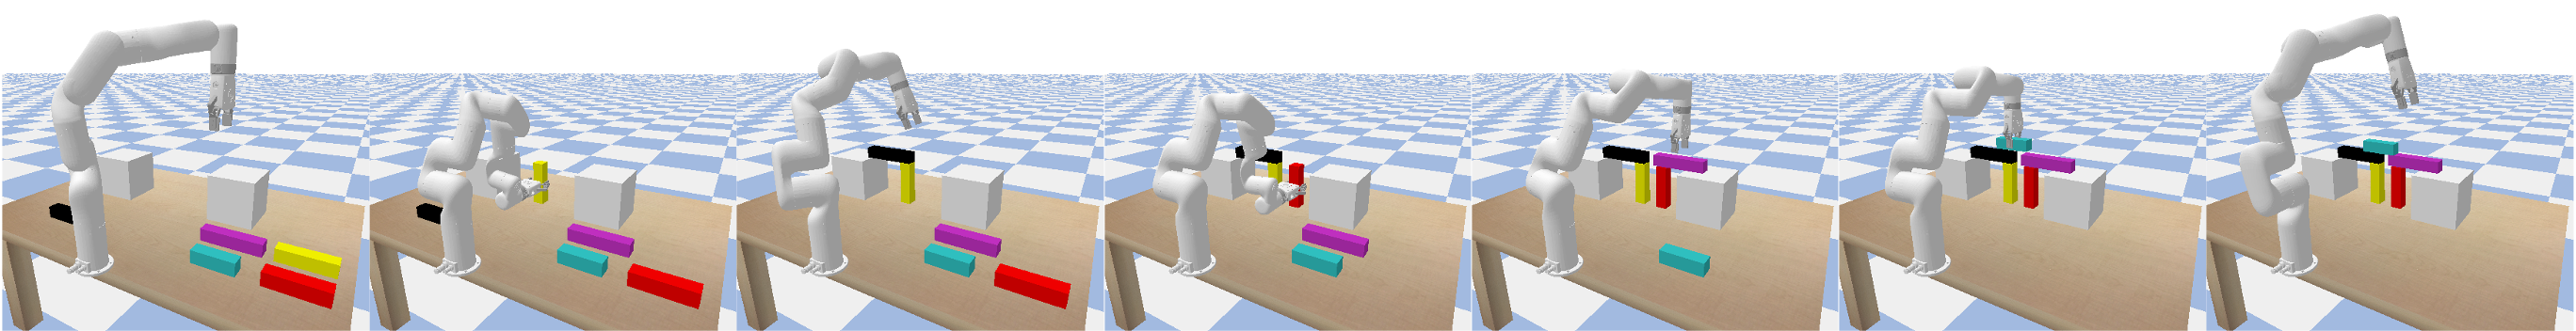}
            \includegraphics[width=\linewidth]{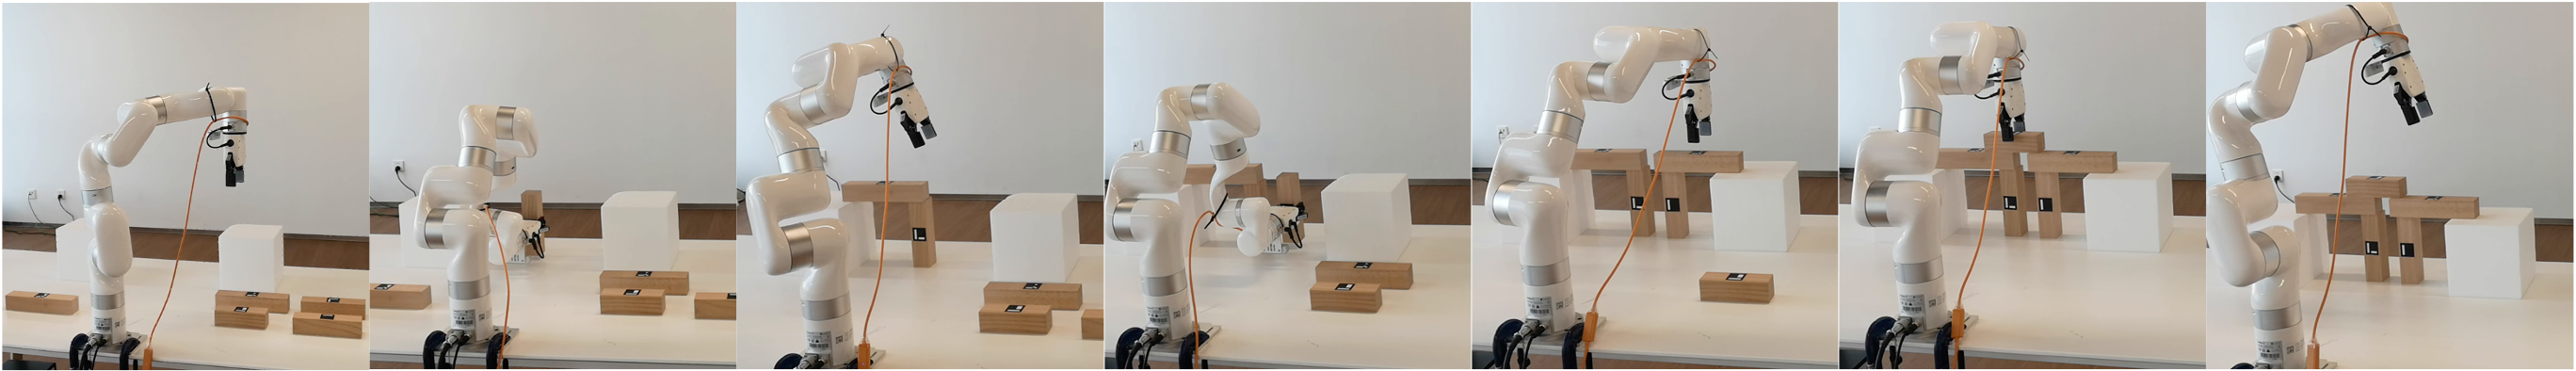}
            % \caption{}
            % \label{fig:policy_5b}
        \end{subfigure}
    \end{minipage}
    \caption{Learned strategies can generalize to different cliff widths and building block sizes.}
\end{figure*}
}
